# Supplementary material for: The Power of Choice in Priority Scheduling
Source: arXiv:1706.04178 source file (2017-06-13)
Supplement: Supplementary file 1 [file appendix.tex]

%!TEX root = paper.tex
\appendix
